# Supplementary material for: Hyperpolarisation Dynamics: Asymptotic Polarisation
Source: arXiv:2404.07578 ancillary file (2024-04-11)
Supplement: Supplementary file 1 [file Supplementary_Info.pdf]

# Supplementary Information

The following derivation is outlined for the case of a nitrogen vacancy (NV) center coupled to $^{13}$C nuclear spins in diamond, although the concepts are broader and may be applied to any central electronic qubit coupled to nuclear spins. The pure-dephasing Hamiltonian for a NV system under microwave (MW) driving coupled to multiple nuclear spins takes the form $\hat{H}(t) = \hat{H}_0 + \hat{H}_p(t)$:

$$\hat{H}_0 = \sum_{n=0}^{N_{\rm nuc}} \left[ \omega_L \hat{I}_z^{(n)} + \hat{S}_z (A_z^{(n)} \hat{I}_z^{(n)} + A_x^{(n)} \hat{I}_x^{(n)}) \right] \tag{1}$$

where $\omega_L = -\gamma_C B_0$ with a $^{13}$C gyromagnetic ratio for $\gamma_C$, $A_i^{(n)}$ are $i^{\rm th}$ components of the hyperfine coupling strength relative to the NV $z$-axis between the $n^{\rm th}$ nuclei and the central spin, $\hat{S}_i$ are in the qubit basis, chosen to be $\{|0\rangle, |\pm 1\rangle\}$ and $\hat{I}_i^{(n)}$ are the $n^{\rm th}$ nuclear spin-1/2 operators. Hyperfine couplings throughout this study are taken from the realistic cluster in [1, 2]. The pulse Hamiltonian in the rotating frame of the microwave field is $\hat{H}_p(t) = \Omega_x(t)\hat{S}_x + \Omega_y(t)\hat{S}_y$ where $\Omega_{x,y}(t)$ are the waveforms of the MW control field for the $x, y$ pulses. The magnetic field is assumed to align with the NV $z$-axis. Throughout this appendix it is taken that $\hbar = 1$.

The operator $\hat{S}_z$ is not equivalent to the corresponding Pauli matrix as it is in the subspace of a spin-1 operator. Simplifications can be made by decomposing the operator in terms of Paul-matrix operators as $\hat{S}_z = \pm(\mathbb{I} - \hat{\sigma}_z)/2$. Additionally, rather than taking the nuclear spins to be in the frame of the NV axis, they can be transformed into the average basis for each spin. The transformed Hamiltonian is then

$$\hat{H}_0 = \sum_{n=0}^{N_{\rm nuc}} \left[ \omega_I^{(n)} \hat{I}_z^{(n)} + \hat{S}_z (A_\perp^{(n)} \hat{I}_x^{(n)} + A_\parallel^{(n)} \hat{I}_z^{(n)}) \right] \tag{2}$$

where the nuclear basis axes have been transformed to $\mathbf{e}_z \to \sin\theta_l^{(n)}\,\mathbf{e}_x \mp \cos\theta_l^{(n)}\,\mathbf{e}_z$ and $\mathbf{e}_x \to \cos\theta_l^{(n)}\,\mathbf{e}_x \pm \sin\theta_l^{(n)}\,\mathbf{e}_z$ such that $\omega_I^{(n)} = \sqrt{(\omega_L \pm A_z^{(n)}/2)^2 + (A_x^{(n)}/2)^2}$ and $\theta_l^{(n)} = A_x^{(n)}/(2\omega_L \pm A_z^{(n)})$. The new hyperfine couplings are then $A_\parallel^{(n)} = A_x^{(n)} \sin\theta_l^{(n)} \mp A_z^{(n)} \cos\theta_l^{(n)}$ and $A_\perp^{(n)} = A_x^{(n)} \cos\theta_l^{(n)} \pm A_z^{(n)} \sin\theta_l^{(n)}$ and without loss of generality, we re-label the couplings in the Hamiltonian back to $A_\perp \to A_x$ and $A_\parallel \to A_z$. The NV spin operator is now pseudo-spin-1/2 equal to $\hat{S}_z = \hat{\sigma}_z/2$, in the same basis, we label $\{|0\rangle = |u\rangle, |\pm 1\rangle = |d\rangle\}$ as this Hamiltonian is general for pseudo-spin-1/2 electronic spins. Without loss of generality, we choose the $m_s = -1$ state.

## PULSEPOL HAMILTONIAN

The waveform of the MW control field is dependent on the DD protocol which is applied. PulsePol is a DD protocol used for dynamic nuclear polarisation (DNP), as it is state selective. The form of this pulse protocol is displayed in Fig.1 in the main paper. The Rabi-frequency due to the microwave drive is denoted $\Omega$. This protocol is periodic with period $T = 4\tau$ and is applied for a total time of $T_{\rm tot} = 8N_p\tau$. Although the protocol period is $T$, the actual period is defined as $2T$. This convention will be taken here for reasons seen later.

Using the waveform of the DD control field, the system can be transformed into the rotating frame of the microwave control field using the reference Hamiltonian $\hat{H}_{\rm ref}(t) = \hat{H}_p(t)$, also known as the *toggling frame*. The transformation to this frame requires the time evolution operator $\hat{U}_p(t)$ to be constructed. While this may be difficult for general time-dependent Hamiltonians, for instantaneous pulses this can be constructed piecewise, such that at time $t$ between the $m$ and $m+1$ pulse:

$$\hat{U}_p(t) = \mathcal{T}\left\{ \prod_{i=0}^{m} \hat{R}_{\mathbf{n}_m}(\theta_m) \right\} \tag{3}$$

where $\hat{R}_{\mathbf{n}_m}(\theta_m)$ is a rotational transformation by angle $\theta_m$ around the central spin axis $\mathbf{n}_m$ for the $m^{\rm th}$ pulse and the transformed Hamiltonian is $\hat{H}'(t) = \hat{U}_p^\dagger(t)\hat{H}_0\hat{U}_p(t)$. None of these transformations affect the nuclear basis as the MW control field targets the central spin only, hence the transformation can be rewritten $\hat{H}'(t) = \hat{H}_I + \hat{U}_p^\dagger(t)\hat{S}_z\hat{U}_p(t) \otimes \hat{V}$

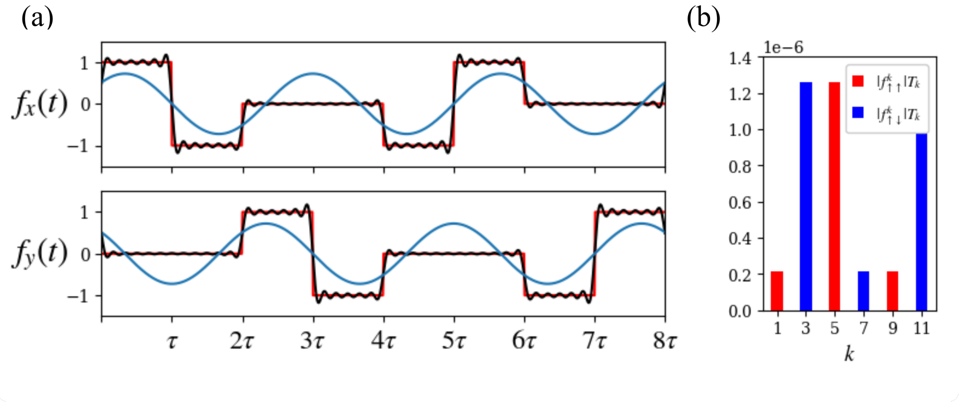


FIG. 1. A graphical representation of the PulsePol modulation functions over a single period $2T = 8\tau$. (a) shows the time series of each modulation function $f_{x,y}(t)$ plotted in red alongside the superposition of Fourier modes up to $k = 50$ in black. This highlights that the true periodicity of the modulation functions is $2T$, not $T$. One particular Fourier mode, $k = 3$ is plotted with frequency $\omega_3 = 3\pi/T$. (b) shows the Fourier amplitudes of $f^k_{\uparrow\uparrow} = f^k_x + if^k_y$ (red) and $f^k_{\uparrow\downarrow} = f^k_x - if^k_y$ (blue), scaled by $T_k = k\pi/\omega_I$.

where we define $\hat{V} = A_z^{(n)}\hat{I}_z^{(n)} + A_x^{(n)}\hat{I}_x^{(n)}$ and $\hat{H}_I = \omega_I^{(n)}\hat{I}_z^{(n)}$ for the $n^{\text{th}}$ nuclear spin. As the unitary transformation operator is discrete in time, so is the resulting transformed Hamiltonian. Due to the periodicity of DD protocols, it is expected that by design $\hat{U}_p(2N_pT) = \mathbb{I}$.

The pulses perform sequential discrete basis changes on central spin operators, so $\hat{S}_z$ in the toggling frame can be written $\hat{S}_z(t) = \sum_{i=x,y,z,} f_i(t)\hat{S}_i$, where $f_i(t)$ are known as modulation functions and it is expected that $\hat{S}_z(2T) = \hat{S}_z$. This would not be fulfilled if total period is not $2T$ as $\hat{S}_z(T) = -\hat{S}_z$. The Hamiltonian in this frame can then be written as

$$\hat{H}(t) = \sum_{n=0}^{N_{\text{nuc}}} \left[ \omega_I^{(n)}\hat{I}_z^{(n)} + \sum_{i=x,y,z} f_i(t)\hat{S}_i \left(A_z^{(n)}\hat{I}_z^{(n)} + A_x^{(n)}\hat{I}_x^{(n)}\right) \right]. \tag{4}$$

Using the piecewise construction of $\hat{U}_p(t)$ defined in Eq.(3), the modulation functions for PulsePol are found to be:

$$f_x(t) = \begin{cases} 1 \text{ for } 0 < t < \tau \text{ and } 5\tau < t < 6\tau \\ -1 \text{ for } \tau < t < 2\tau \text{ and } 4\tau < t < 5\tau \\ 0 \text{ otherwise} \end{cases} \tag{5}$$

and

$$f_y(t) = \begin{cases} 1 \text{ for } 2\tau < t < 3\tau \text{ and } 7\tau < t < 8\tau \\ -1 \text{ for } 3\tau < t < 4\tau \text{ and } 6\tau < t < 7\tau \\ 0 \text{ otherwise} \end{cases} \tag{6}$$

and $f_z(t) = 0$ where these functions are periodic $f_i(t + 2T) = f_i(t)$.

Owing to this periodicity, Fourier decomposition can be used where for $f_x(t)$

$$f_x(t) = \sum_{m=0}^{\infty} \left[a_x^m \cos(\omega_m t) + b_x^m \sin(\omega_m t)\right] \tag{7}$$

defining $\omega_m = m\pi/T$ and where

$$
\begin{aligned}
a_x^m =& \frac{1}{m\pi}\frac{1-(-1)^m}{2}\left[4\sin\left(\frac{m\pi}{4}\right) - 2\sin\left(\frac{m\pi}{2}\right)\right] \\
b_x^m =& \frac{1}{m\pi}\frac{1-(-1)^m}{2}\left[-4\cos\left(\frac{m\pi}{4}\right) + 2\right].
\end{aligned} \tag{8}
$$

The decomposition of the remaining modulation function $f_y(t)$ can be found in a similar fashion, only with coefficients $a_y^m = -(-1)^{\tilde{m}} b_x^m$ and $b_y^m = (-1)^{\tilde{m}} a_x^m$ due to the shift of $t \to t' = t - 2\tau$ in the time dependence where $\tilde{m} = (2m-2)/4$. The time-series of the modulation functions as well as the superposition of a finite number of modes from the Fourier decomposition are shown in Fig.1. We can now see that the modulation functions are actually periodic over $2T$ rather than $T$ due to a remaining difference in phase from $t = 0$ at $t = T$.

The Fourier decomposition can also be made with respect to complex functions $e^{-i\omega_m t}$ where $m \in \mathbb{Z}$. In this case, the Fourier coefficients are related as $f_j^m = a_j^m - ib_j^m$ where $f_j^{-m} = f_j^{m*}$ for $j = x, y$. This relation is only true when $f_j^0 = 0$. These complex functions span the Fourier space of square integrable functions. The three Fourier coefficients can be reduced to two in the following expressions $f_\perp^m = f_x^m + if_y^m$. Figure 1 displays these amplitudes for different values of $m$.

**Magnus Expansion**

If it is assumed that $|A_{x,z}^{(n)}| << 1/T \quad \forall n$, then the time dependence of the Hamiltonian can be resolved in a perturbative fashion using the Magnus expansion. To first order, the evolution operator is approximately $\hat{U}(2T) = \exp[-i2\hat{H}_{\text{avg}}T]$, where $\hat{H}_{\text{avg}}$ is the time period averaged Hamiltonian, constructed as

$$
\hat{H}_{\text{avg}} = \frac{1}{2T}\int_0^{2T} \hat{H}(t)\, dt, \tag{9}
$$

removing the time dependence in place of time averaged field strengths. The assumption of small time scales is assumed for hyperfine coupling terms, but not for fast rotating nuclear precession terms involving $\omega_I^{(n)}$. Commonly, these terms are removed by transforming into the interaction frame of the nuclear spins of interest with reference Hamiltonian $\hat{H}_{\text{ref}}^{(n)} = \omega_I^{(n)}\hat{I}_z^{(n)}$. However, for nuclear spins with different precession frequencies, $\omega_I^{(n)}$, and hence with differing nuclear detunings, this is hard to justify. To include nuclear detunings we instead move into the rotating frame of one of the Fourier modes with reference Hamiltonian $\hat{H}_{\text{ref}} = \omega_k \hat{I}_z^{(n)}$. The Hamiltonian in this frame is then

$$
\hat{H}(t) = \sum_{n=0}^{N_{\text{nuc}}}\left[\delta^{(n)}\hat{I}_z^{(n)} + \sum_{i=x,y} f_i(t)\hat{S}_i\left(A_x^{(n)}\hat{I}_x^{(n)}(t) + A_z^{(n)}\hat{I}_z^{(n)}\right)\right] \tag{10}
$$

where $\hat{I}_x^{(n)}(t) = \cos(\omega_k t)\hat{I}_x^{(n)} - \sin(\omega_k t)\hat{I}_y^{(n)}$ and the nuclear detunings $\delta^{(n)} = \omega_I^{(n)} - \omega_k$. To ensure that $|\delta^{(n)}| \ll 1/T$, we assume that the chosen pulse spacing $T$ is such that $\omega_k = k\pi/T \simeq \omega_L$.

Owing to the fact that the Fourier modes form a complete set of basis states, all terms in the Fourier series of the modulation functions for $m \neq k$ are zero to this order of Magnus expansion. Choosing the mode $k = 3$ shown in Fig.1 with $T \simeq 3\pi/\omega_L$, the first order Hamiltonian is found to be:

$$
\hat{H}_{\text{avg}} = \sum_{n=0}^{N_{\text{nuc}}}\left[g^{(n)}(\hat{S}_+\hat{I}_-^{(n)} + \hat{S}_-\hat{I}_+^{(n)}) + \delta^{(n)}\hat{I}_z^{(n)}\right] \tag{11}
$$

where we assume the Hamiltonian is an independent sum of $N_{\text{nuc}}$ spins, with all interactions mediated by the central electronic spin. We define $g^{(n)} = A_x^{(n)}\alpha/4$, $\alpha = 2(\sqrt{2}+2)/3\pi$. As stated previously, this Hamiltonian is appropriate for small detunings $|\delta^{(n)}| \ll 1/T$. If this is not satisfied, higher order terms may be needed. Note that the protocol period is said to be resonant with the $n^{\text{th}}$ nuclear spin (labelled as $T_r^{(n)}$) at resonance $\omega_k = k\pi/T_r^{(n)} = \omega_I^{(n)}$ for the $k^{\text{th}}$ harmonic. This result is identical to that in [3].

## MARKOV CHAINS

In order to understand the stationary distribution of the repeated nuclear spin polarisation, we will employ a Markov chain model. In this section we outline the Markov chain description of a stochastic process.

A Markov chain is a discrete time stochastic process with a finite number of states, where the probability of transition between two particular states has no hysteresis. Explicitly, the probability of transition only depends on the previous time step's state with no memory of past time steps. Hence, for a random variable at time $X_t$, the probability of measuring it to be $x_t$ at this time step is

$$P(X_t = x_t | X_{t-1} = x_{t-1}, ..., X_0 = x_0) = P(X_t = x_t | X_{t-1} = x_{t-1}). \tag{12}$$

The probability of being in a state $n \in \mathbb{Z}^+$ at a discrete time $t_2$ is then

$$p(n, t_2) = \sum_m p(n, t_2 | m, t_1) p(m, t_1) \tag{13}$$

which can be represented in vector form $\mathbf{p}(t_2) = (..., p(n, t_2), p(n+1, t_2), ...)^T$. Then, Eq.(13) can be written as

$$\mathbf{p}(t_{R+1}) = Q\mathbf{p}(t_R) = Q^{(R+1)}\mathbf{p}_0 \tag{14}$$

where $Q_{mn} = p(n, t_{R+1} | m, t_R)$ is the so called *transition matrix*. The probability vectors are normalised in a probabilistic sense, or $\sum_n p(n, t_R) = 1$, and each element of the vector is positive definite $p(n, t_R) \geq 0 \ \forall \ R, n$. The transition matrix is a *stochastic* matrix, meaning that all entries are also positive definite $Q_{nm} \geq 0 \ \forall \ n, m$ and the sum of all probabilities exiting a site sum to unity, or $\sum_n Q_{nm} = 1 \ \forall \ m$. This is a useful construction, as it allows steady states of the system to be readily determined as follows.

If $Q$ has an eigenstate $\mathbf{v}_n$, with an eigenvector $\lambda_n = 1$, then this normalised state is a steady state of the system, such that $Q\mathbf{v}_n = \mathbf{v}_n$. For an *irreducible* Markov process, or a system that has no terminal states (states where no population leaves at any time step), this condition is stronger and all other eigenvalues must lie within a unit disc in the complex plane, or $|\lambda_{m \neq n}| < 1 \ \forall \ m$. Hence, by finding the eigenvalues of the transition matrix, an indication of stationary distribution of the system can be found.

The full dynamics of a general state can be also constructed using the eigenvector decomposition of the initial state, such that the initial probability distribution vector is $\mathbf{p}(0) = \sum_n c_n(0)\mathbf{v}_n$ where $c_n(0)$ are the expansion coefficients with respect to the eigenbasis of $Q$. Then, the evolution of the probability distribution vector in this basis is

$$\mathbf{p}(t_R) = \sum_n c_n(0) Q^R \mathbf{v}_n = \sum_n \lambda_n^R c_n(0) \mathbf{v}_n. \tag{15}$$

For an irreducible Markov process, it is now clear what the stationary distribution is. Any eigenvector with eigenvalue $|\lambda_n| < 1$ will asymptotically tend to zero as $R \to \infty$, whereas the eigenvector $\mathbf{v}_k$ with $|\lambda_k| = 1$ will not. Hence, when the system reaches an equilibrium it is the stationary distribution, or more formally, $\lim_{t\to\infty} \mathbf{p}(t_R) = \mathbf{v}_k$. We will now find the stationary distribution of a general two state system.

### Two State Chain

The simplest non-trivial Markov chain, which we study here, is one with two states $n = 0, 1$. For reasons seen later, we label these two states $n_0 \equiv n_\uparrow$ and $n_1 \equiv n_\downarrow$. Assuming that the graph for the Markov chain is fully connected, as shown in Fig.3 in the main paper, then the transition matrix is

$$Q = \begin{pmatrix} 1 - r_- & r_+ \\ r_- & 1 - r_+ \end{pmatrix} \tag{16}$$

where $r_\pm$ are the transition probabilities between $n_{\uparrow/\downarrow}$ states at each time step. This is an irreducible Markov chain and will have a stationary distribution of one eigenvector with an eigenvalue of 1. The eigenvectors and eigenvalues of this matrix are

$$\mathbf{v}_1 = \frac{1}{r_+ + r_-}\begin{pmatrix} r_+ \\ r_- \end{pmatrix}, \quad \lambda_1 = 1 \tag{17}$$

$$\mathbf{v}_2 = \frac{1}{2}\begin{pmatrix} 1 \\ -1 \end{pmatrix}, \quad \lambda_2 = 1 - r_- - r_+. \tag{18}$$

Then, as before, an initial state of $\mathbf{p}(0) = (p_\uparrow^{(0)}, p_\downarrow^{(0)})^{\mathrm{T}}$ where $p_\uparrow^{(0)} + p_\downarrow^{(0)} = 1$ can be decomposed into the eigenbasis of $Q$, such that $\mathbf{p}(0) = c_1(0)\mathbf{v}_1 + c_2(0)\mathbf{v}_2$. For this initial state, the expansion coefficients can be found to be $c_1 = 1$ and

$$c_2(0) = \mathcal{P}_0 - \frac{r_+ - r_-}{r_+ + r_-}. \tag{19}$$

where $\mathcal{P}_0 = p_\uparrow^{(0)} - p_\downarrow^{(0)}$. We will now motivate the use of a Markov chain model in the context of repeated DNP of a single nuclear spin via an electronic spin and apply this framework.

### Semi-Classical Approximation

As mentioned in the previous chapter, a common method of obtaining a high level of polarisation involves sequentially pushing the nuclear spin into a pure polarised state by interweaving packets of coherent dynamics with electronic central spin re-initialisation. Explicitly, PulsePol was considered for duration $T_{\mathrm{tot}} = 2N_pT$ with re-initialisation of the central spin $R$ times. Here, we will mostly ignore the specifics of coherent dynamics within each repetition and will study the accumulation of polarisation at each repetition. Take the central spin to be initialised into the $|u\rangle$ state, but the nuclear spin in a general mixture with $p_\uparrow^{(R)}$ in the $|\uparrow\rangle$ state and $p_\downarrow^{(R)}$ in the $|\downarrow\rangle$ state. The initial density matrix is then $\rho^{(R)}(0) = \rho_\uparrow \otimes (p_\uparrow^{(R)}\rho_\uparrow + p_\downarrow^{(R)}\rho_\downarrow)$ with

$$\rho_\uparrow = \begin{pmatrix} 1 & 0 \\ 0 & 0 \end{pmatrix}, \quad \rho_\downarrow = \begin{pmatrix} 0 & 0 \\ 0 & 1 \end{pmatrix}. \tag{20}$$

The operation of re-intialisation on the central spin is defined as

$$\rho^{(R+1)}(0) = \rho_\uparrow \otimes \mathrm{Tr}_c(\rho^{(R)}(T_{\mathrm{tot}})) \tag{21}$$

where $\mathrm{Tr}_c()$ is the partial trace over the central spin state space. Taking the coherent dynamics to evolve according to $\hat{U}(t)$, after $t = T_{\mathrm{tot}} = 2N_pT$ followed by re-initialisation of the central spin, the distribution of the system is

$$\begin{aligned}\rho^{(R+1)}(0) = \rho_\uparrow \otimes \Big[&\mathrm{Tr}_c(\hat{U}(T_{\mathrm{tot}})(\rho_\uparrow \otimes \rho_\uparrow)\hat{U}^\dagger(T_{\mathrm{tot}}))p_\uparrow^{(R)} \\ &+ \mathrm{Tr}_c(\hat{U}(T_{\mathrm{tot}})(\rho_\uparrow \otimes \rho_\downarrow)\hat{U}^\dagger(T_{\mathrm{tot}}))p_\downarrow^{(R)}\Big].\end{aligned} \tag{22}$$

We assume the equation above can be written as $\rho^{(R+1)}(0) = \rho_\uparrow \otimes (\rho_\uparrow p_\uparrow^{(R+1)} + \rho_\downarrow p_\downarrow^{(R+1)})$. In essence this is a *semi-classical* approximation, assuming that the accumulation of polarisation at each repetition is a classical process and that the nuclear spin cannot evolve into a separable (from the central spin state space) superposition state. The resulting density matrix is then diagonal in the nuclear state space. If this assumption holds, the time evolution components of Eq.(22) can be written

$$\mathrm{Tr}_c(\hat{U}(T_{\mathrm{tot}})(\rho_\uparrow \otimes \rho_\uparrow)\hat{U}^\dagger(T_{\mathrm{tot}})) = (1 - r_-)\rho_\uparrow + r_-\rho_\downarrow \tag{23}$$

$$\mathrm{Tr}_c(\hat{U}(T_{\mathrm{tot}})(\rho_\uparrow \otimes \rho_\downarrow)\hat{U}^\dagger(T_{\mathrm{tot}})) = r_+\rho_\uparrow + (1 - r_+)\rho_\downarrow \tag{24}$$

in the nuclear state space. Then, the updated probabilities after each repetition are

$$p_\uparrow^{(R+1)} = (1 - r_-)p_\uparrow^{(R)} + r_+p_\downarrow^{(R)} \tag{25}$$

$$p_\downarrow^{(R+1)} = r_-p_\uparrow^{(R)} + (1 - r_+)p_\downarrow^{(R)}. \tag{26}$$

The expressions above are exactly equivalent to the Markov chain model in Eq.(14) and thus can be written as a vector equation $\mathbf{p}(t_R) = Q^R\mathbf{p}(0)$, where $\mathbf{p}(t_R) = (p_\downarrow^{(R)}, p_\downarrow^{(R)})^{\mathrm{T}}$, $t_R = 2RN_pT$ and $Q$ as a transition matrix. Due to the consistency in notation, $Q$ is of the same form to Eq.(16) and the graphical Markov chain in Fig.3 of the main paper represents this process. The polarisation of this probability distribution is calculated as $\mathcal{P}_R = p_\downarrow^{(R)} - p_\downarrow^{(R)} = \mathrm{Tr}(\sigma_z\mathbf{p}(t_R))$. The evolution of the state, and hence polarisation, after $R$ time steps is constructed using the eigenvectors of $Q$ in Eq.(18) to be

$$\mathcal{P}_R(T) = \mathcal{P}_0(1-\alpha)^R + \frac{r_+ - r_-}{r_+ + r_-}(1-(1-\alpha)^R) \tag{27}$$

for an initial polarisation $\mathcal{P}_0$ where $\alpha = r_+ + r_-$. The expected asymptotic polarisation for the stationary distribution of this Markov chain is then

$$\lim_{R\to\infty}\mathcal{P}_R(T) = \mathcal{P}_\infty(T) = \frac{r_+(T) - r_-(T)}{r_+(T) + r_-(T)}. \tag{28}$$

This describes the semi-classical asymptotic envelope with protocol period $T$ for the repeated polarisation of a single nuclear spin, a key result for this chapter. It is worth noting that pure nuclear state polarisation blocking was neglected when the semi-classical approximation was made. Non-maximal polarisation saturation after 'infinite' repetitions is due to competing polarisation ($r_+$) and de-polarisation ($r_-$) effects, leaving the spin in a non-pure mixed statistical distribution. Hence known as *statistical* polarisation saturation.

## PULSEPOL MARKOV CHAIN

We will now find the asymptotic polarisation envelope for a single nuclear spin using the PulsePol Hamiltonian. The Hamiltonian for a single nuclear spin was derived in the previous chapter to be:

$$\hat{H}_{\mathrm{avg}} = \delta\hat{I}_z + g_+(\hat{S}_+\hat{I}_- + \hat{S}_-\hat{I}_+) \tag{29}$$

for the 3$^{\mathrm{rd}}$ harmonic of PulsePol, where $\delta = \omega_I - \omega_3$ ($\omega_3 = 3\pi/T$), $g_+ \equiv g_3 = (2+\sqrt{2})A_x/(6\pi)$ and $\hat{S}$, $\hat{I}$ are the spin operators of the central spin and nuclear spin respectively. By solving Eq.(23) and (24) with this Hamiltonian, the transition probabilities for the Markov chain model can be found. Using the PulsePol Hamiltonian in Eq.(11), the transition equations are found to be

$$\rho_\uparrow = (1-r_-)\rho_\uparrow + r_-\rho_\downarrow \tag{30}$$

$$|\beta_+(T_{\mathrm{tot}})|^2\rho_\uparrow + [1-|\beta_+(T_{\mathrm{tot}})|^2]\rho_\downarrow = r_+\rho_\uparrow + (1-r_+)\rho_\downarrow \tag{31}$$

where $|\beta_+(t)|^2 = \sin^2(\theta_+)\sin^2(\Omega_+t/2)$ defining $\tan\theta_+ = 2g_+/\delta$ and $\Omega_+ = \sqrt{\delta^2 + 4g_+^2}$. A more complete derivation of these dynamics can be found in [4]. Reading off from the above equations, $r_-(T_{\mathrm{tot}}) = 0$ and $r_+(T_{\mathrm{tot}}) = |\beta(T_{\mathrm{tot}})|^2$. For this Hamiltonian, there is no de-polarisation rate $r_-$ and so the expected asymptotic polarisation envelope from Eq.(28) is $\mathcal{P}_\infty(T) = 1$. Hence, for a general $T_{\mathrm{tot}}$, assuming that $|\delta| \ll 1/T$, it is expected that the polarisation saturates at a maximum value.

Figure 3 and 4 in the main paper tests the analytical expression of $\mathcal{P}_\infty(T)$ against simulations of single nuclear $^{13}$C spin polarisation, namely a nuclear spin with couplings $(A_z, A_x)/2\pi = (-48.6, 9)$ kHz, via a NV center. Saturation at the resonant $T_r = k\pi/\omega_I$ is shown to be maximum $\mathcal{P}(T_r) = 1$ for the simulation, as predicted. However, for $T \neq T_r$ the simulated polarisation saturates below maximum and diverges from $\mathcal{P}_\infty$. This disparity between the analytical expression and the simulation increases the further $T$ is from the resonant value, or the for larger values of $\delta$.

In addition, Fig.3 in the main paper demonstrates dramatic loss of polarisation symmetrically distributed about the resonant $T_r$ in both the single spin simulation and Markov model. These are often termed as 'side-dips' in the polarisation [4]. For the Markov model, the polarisation in Eq.(28) is zero if, as well as $r_- = 0$, the polarisation rate $r_+ = 0$. This condition is met when $T = T_{\mathrm{dip}}$ which satisfies

$$\begin{aligned} T_{\mathrm{dip}} &= \frac{T_r}{(1+\mu^2)}\left[1 + \frac{n}{kN_p}\sqrt{1+\mu^2\left(\frac{k^2N_p^2}{n^2} - 1\right)}\right] \\ &\simeq T_r\left[1 \pm \frac{n}{kN_p}\right] \end{aligned} \tag{32}$$

where $n \in \mathbb{Z}$, $n \neq 0$, is the $n^{\text{th}}$ side dip, $k$ is the resonance harmonic and $\mu = 2g_+/\omega_I$.

The average PulsePol Hamiltonian does not capture the full single spin simulation away from the resonant value $T_r$, where $\omega_I = \omega_3$ and the detuning $\delta = 0$. For larger values of this detuning the assumption $|\delta| \ll 1/T$ may not be satisfied and higher order terms are required. In the next section we will explore the higher order terms for this Hamiltonian, demonstrating how they contribute to the polarisation saturation seen in single nuclear spin simulations.

## Higher Order Effects

When deriving the PulsePol Hamiltonian previously, the Magnus expansion was truncated to first order, assuming that $|\delta|, A_x \ll 1/T$. However, for larger detuning from the resonant periodicity $T_r$ the Hamiltonian was shown not align with simulations as there is no apparent de-polarisation mechanism. Larger values of detuning, $\delta$, may break the assumption $|\delta| \ll 1/T$ and so the first order approximation may be too naïve. We now consider second order terms in the PulsePol Hamiltonian.

It was shown to first order that all Fourier modes $m$ in the Fourier decomposition of the modulation functions that are not the chosen mode $k$ are zero. Where the parameter range was chosen such that $\omega_k = k\pi/T \simeq \omega_I$. For second order terms, this may not be the case and other Fourier modes with $m \neq k$ could contribute. To include these we consider higher order terms of the Magnus expansion.

The second order term of the Magnus expansion is

$$\hat{H}^{(2)} = \frac{1}{4iT} \int_0^{2T} dt_1 \int_0^{t_1} dt_2 [\hat{H}(t_1), \hat{H}(t_2)]. \tag{33}$$

There are a multitude of terms in this Hamiltonian, especially when including all terms in the Fourier decomposition. However, assumptions can be made to simplify this. We assume that the perpendicular coupling of the nuclear spin is small, $A_x \ll 1/T$, such that any terms of order $A_x^2$ or above are negligible. Although, noticing that the saturation is off-resonance, we relax the condition that $\delta$ is small, and higher order terms involving larger powers of $\delta$ will be considered. Formally, we assume all terms $[\hat{H}_m, \hat{H}_k]$ for odd $m, k$ are negligible with only higher order contributions $[\delta \hat{I}_z, \hat{H}_m]$ included.

If the Fourier mode $m = k$ is chosen for the first order Hamiltonian, then second order perturbations will be framed as $l$-‘photon’ effects with terms $m = k + 2l$ in the Fourier series, where $l \in [-\tilde{k}, \infty)$ and defining $\tilde{k} = (k-1)/2$. We define $m$ in terms of $2l$ as only odd $m$ terms in the Fourier series are non-zero. First we consider zero-‘photon’ effects with $l = 0$, or $m = k$. Collecting terms $\propto \delta \hat{I}_z \hat{H}_k$ from Eq.(33), the second order Hamiltonian of this subset is

$$\hat{H}_k^{(2)} = \frac{g_k \delta}{\omega_k} \left[ \frac{1 - (-1)^{\tilde{k}}}{2} \hat{H}_{\uparrow\uparrow} - \frac{1 + (-1)^{\tilde{k}}}{2} \hat{H}_{\uparrow\downarrow} \right] \tag{34}$$

where the effective coupling $g_k = \sqrt{2} A_x b_x^k / 4$, $\hat{H}_{\uparrow\uparrow} = (\hat{S}_+ \hat{I}_+ + \hat{S}_- \hat{I}_-)/2$ and $\hat{H}_{\uparrow\downarrow} = (\hat{S}_+ \hat{I}_- + \hat{S}_- \hat{I}_+)/2$. Note that this is proportional to $\delta/\omega_1$, where $\omega_1$ sets the energy scale between Fourier terms. For $k = 3$, this introduces a de-polarisation term $\hat{H}_3^{(2)} \propto \hat{H}_{\uparrow\uparrow}$.

Now consider multi-‘photon’ effects, $l \neq 0$. Here, we collect terms $\propto \delta \hat{I}_z \hat{H}_m$ for $m \neq k$ in Eq.(33), yielding second order corrections $\sum_{l=-\tilde{k}}^{\infty} \hat{H}_{kl}^{(2)}$ where

$$\hat{H}_{kl}^{(2)} \simeq \frac{g_{k+2l} \delta}{\omega_1} \left[ \frac{2l + (1 + (-1)^{\tilde{k}+l}) k}{2l(l+k)} \hat{H}_{\uparrow\uparrow} - \frac{2l + (1 - (-1)^{\tilde{k}+l}) k}{2l(l+k)} \hat{H}_{\uparrow\downarrow} \right] \tag{35}$$

excluding $l = 0$. Note that as $|l|$ grows, the contribution of these terms to the Hamiltonian diminishes as $||\hat{H}_{kl}^{(2)}|| \propto 1/l$. Hence, although there are an infinite number of terms, large $l$ terms can be effectively neglected.

To second order in the Magnus expansion, the Hamiltonian $\hat{H}_k^{[2]} \simeq \hat{H}_{\text{avg}} + \hat{H}_k^{(2)} + \sum_{l=-\tilde{k}}^{\infty} \hat{H}_{kl}^{(2)}$ and $l \neq 0$. Returning to the commonly studied PulsePol harmonic $k = 3$ and assuming that terms $|l| > 1$ are negligible, the Hamiltonian to second order is

$$\begin{aligned} \hat{H}_3^{[2]} \simeq \delta \hat{I}_z &+ g_+(\hat{S}_+\hat{I}_- + \hat{S}_-\hat{I}_+) \\ &+ g_-(\hat{S}_+\hat{I}_+ + \hat{S}_-\hat{I}_-) \end{aligned} \tag{36}$$

where

$$g_+ \simeq g_3 + \frac{3\delta}{8\omega_3}(2g_1 - g_5) \tag{37}$$

and

$$g_- \simeq \frac{\delta}{2\omega_3}(g_3 + 3g_1 + 3g_2) \tag{38}$$

We now drop the superscript '[2]' from the Hamiltonian for convenience. The addition of these higher order terms to the Hamiltonian has allowed de-polarisation, proportional to $g_-$ and thus the nuclear detuning $\delta$ as required.

The new $\delta$-dependent terms in this Hamiltonian break the eigenstate $|u\uparrow\rangle$, allowing evolution into the $|d\downarrow\rangle$ state. The matrix representation of the Hamiltonian in Eq.(36) is

$$\hat{H}_3 = \begin{matrix} |u\uparrow\rangle \\ |d\downarrow\rangle \\ |d\uparrow\rangle \\ |u\downarrow\rangle \end{matrix} \begin{pmatrix} \delta/2 & g_- & 0 & 0 \\ g_- & -\delta/2 & 0 & 0 \\ 0 & 0 & \delta/2 & g_+ \\ 0 & 0 & g_+ & -\delta/2 \end{pmatrix} \tag{39}$$

The two states $|u\downarrow\rangle$ and $|d\uparrow\rangle$ form a pseudospin 1/2 model with identical form to the first order Hamiltonian, only with a slightly altered coupling $g_+$. The same form of transition rates will be taken, with $g \to g_+$ defined here. The remaining subspace $\{|u\uparrow\rangle, |d\downarrow\rangle\}$ also forms a pseudo-spin 1/2 model. The eigenstates and eigenvalues for this subspace are

$$|\chi_1\rangle = \cos\left(\frac{\theta_-}{2}\right)|u\uparrow\rangle + \sin\left(\frac{\theta_-}{2}\right)|d\downarrow\rangle, \quad \epsilon_1 = \frac{\omega_-}{2} \tag{40}$$

$$|\chi_2\rangle = \cos\left(\frac{\theta_-}{2}\right)|d\downarrow\rangle - \sin\left(\frac{\theta_-}{2}\right)|u\uparrow\rangle, \quad \epsilon_2 = -\frac{\omega_-}{2} \tag{41}$$

where $\omega_- = \sqrt{\delta^2 + 4g_-^2}$ and $\tan\theta_- = 2g_-/\delta$. If $\delta = 0$, the eigenstates are the Zeeman states $\{|u\uparrow\rangle, |d\downarrow\rangle\}$ as with the first order Hamiltonian. However, for non-zero $\delta$ the polarised state $|u\uparrow\rangle$ can transition into the non-polarised state $|d\downarrow\rangle$.

Returning to the Markov chain model, the transition equations are updated for this second order Hamiltonian to

$$[1 - |\beta_-(T_{\text{tot}})|^2]\rho_\uparrow + |\beta_-(T_{\text{tot}})|^2\rho_\downarrow = (1 - r_-)\rho_\uparrow + r_-\rho_\downarrow \tag{42}$$

$$|\beta_+(T_{\text{tot}})|^2\rho_\uparrow + [1 - |\beta_+(T_{\text{tot}})|^2]\rho_\downarrow = r_+\rho_\uparrow + (1 - r_+)\rho_\downarrow \tag{43}$$

where $|\beta_\pm(t)|^2 = \sin^2\theta_\pm \sin^2(\Omega_\pm t/2)$ with the Rabi-frequencies $\Omega_\pm = \omega_\pm = \sqrt{\delta^2 + 4g_\pm^2}$. The transition probabilities are then read off to be $r_\pm(T_{\text{tot}}) = |\beta_\pm(T_{\text{tot}})|^2$. As expected, now $r_- \neq 0$, allowing for de-polarisation.

In the main paper, Fig.3 and 4 compare the Markov model in Eq.(28) using the second order transition rates in Eq.(36) against simulations of a single $^{13}$C nuclear spin polarisation via a NV center. For a weakly coupled nuclear spin in Fig.3 the second order Markov model replicates full simulations well, especially for smaller $\delta$. As $\delta$ grows, the analytical model diverges, where higher order terms $> 2$ are needed. For standard nuclear detuning $\delta/2\pi \sim 30\,\text{kHz}$, this model will suffice.

Moreover, Fig.4 in the main paper demonstrates the asymptotic polarisation envelope for a strongly coupled nuclear spin with couplings $(A_z, A_x)/2\pi = (-11.4, 59.2)\,\text{kHz}$. The analytical model also captures the full simulation well for

the range of $\delta$ we are interested in; however, both simulation and model illustrate a different envelope to the weaker nuclear spin, where the polarisation side dips are much broader and converge to $\mathcal{P}_\infty(T_{\text{dip}}) = -1$. As well, in the vicinity of the side dips maximum polarisation of $\mathcal{P}_\infty = 1$ is recovered. To explain this, consider the expression for side dips in Eq.(32). Initially, this condition was introduced for $r_+ = 0$, but now $r_- \neq 0$. There are now two conditions which are not necessarily degenerate, a polarisation dip when $r_+ = 0$ and a polarisation peak when $r_- = 0$. Such conditions are met when

$$T_{\text{dip}}^{\pm} = \frac{T_r}{(1+\mu_\pm^2)}\left[1 + \frac{n}{kN_p}\sqrt{1+\mu_\pm^2\left(\frac{k^2N_p^2}{n^2} - 1\right)}\right] \tag{44}$$

where $n \in \mathbb{Z}$ and $\mu_\pm = g_\pm/\omega_I$, noting that $g_+ \propto A_x$ and $g_- \propto \delta A_x$. For a nuclear spin coupled with $A_x \ll \omega_I$, or $\mu \ll 1$, both conditions are degenerate and $T_{\text{dip}}^{\pm} \simeq T_r[1+\frac{n}{kN_p}]$ where $\mathcal{P}_\infty(T_{\text{dip}}^{\pm}) = 0$, as is the case in Fig.3 in the main paper. However, larger $A_x$ corrections to $T_{\text{dip}}^{+}$ of $\mu_+ \propto A_x/\omega_I$ may shift this value, whilst $T_{\text{dip}}^{-}$ remains unshifted as $\mu_- \propto |\delta|A_x/\omega_I \ll 1$. Hence, there may be two separate conditions for $r_- = 0$, where $\mathcal{P}_\infty(T_{\text{dip}}^{-}) = 1$ and $r_+ = 0$, where $\mathcal{P}_\infty(T_{\text{dip}}^{+}) = -1$, as illustrated in Fig.4 in the main paper for a nuclear spin with $A_x/2\pi \simeq 60\,\text{kHz}$.

A nuclear spin with detuning $\delta/2\pi \sim 30\,\text{kHz}$ and perpendicular coupling $A_x/2\pi \simeq 10\,\text{kHz}$ will have a loss of $\sim 5\%$ fidelity during initialisation for DNP at the standard Larmor frequency and a modest magnetic field of $B_0 \simeq 400\,\text{G}$. This loss in fidelity may be more drastic for stronger coupled spins due to broader side dips, as seen in Fig.4.

## CONTINUUM LIMIT: MASTER EQUATION

We now take the continuum limit of the repeated polarisation in order to include $T_1$ relaxation times of nuclear spin states. Although not important for local spins, this will help give an estimate for the total number of nuclear spins in the vicinity to the central spin which polarise. A general Markov model in Eq.(13) can be re-written as

$$p_n(t+\Delta t) - p_n(t) = \sum_m W_{m\to n}\Delta t\, p_m(t) - \left(\sum_m W_{n\to m}\Delta t\right) p_n(t) \tag{45}$$

where $\Delta t$ is the time step between transitions and $W_{m\to n}$ are the transition rates, defined as $W_{m\to n}\Delta t = Q_{mn}$. If the transition probabilities per time step are small, such that $Q_{nm} \ll 1\,\forall n, m$ then the continuum limit of $\Delta t \to 0$ can be taken to give

$$\partial_t p_n(t) = \sum_m W_{m\to n}\, p_m(t) - \sum_m W_{n\to m} p_n(t) \tag{46}$$

known as the *master equation*. Here $\partial_t p \equiv \frac{\partial p}{\partial t}$.

For our single nuclear spin system system, we introduce the spatial dependence of the hyperfine couplings, such that $\omega_I(\mathbf{r}) = \sqrt{(\omega_L - A_z(\mathbf{r})/2)^2 + (A_x(\mathbf{r})/2)^2}$ and $g_\pm \propto A_x(\mathbf{r})$, where $\mathbf{r} = x\mathbf{e}_x + y\mathbf{e}_y + z\mathbf{e}_z$. The formula for the spatial dependence of $\mathbf{A}(\mathbf{r})$ couplings is

$$\begin{aligned}\mathbf{A}(\mathbf{r}) = &-\frac{\mu_0}{4\pi}\frac{\gamma_e\gamma_C}{r^3}\left(\frac{3\sin 2\theta\cos\phi}{2}, \frac{3\sin 2\theta\sin\phi}{2}, 3\cos^2\theta - 1\right) \\ =&(A_x, A_y, A_z).\end{aligned} \tag{47}$$

Additionally, a global magnetic field inhomogeneity could be included by allowing $\omega_L(\mathbf{r}) = -\gamma_n B_0(\mathbf{r})$, but we will assume that the magnetic field is homogeneous on the scales used here. Transition rates are now dependent on the nuclear spin's orientation to the central spin and the periodicity of the protocol, $r_\pm(\mathbf{r}, T_{\text{tot}} = 2N_pT)$. Often when polarising multiple nuclear spins, a DNP protocol is applied to match the Larmor frequency of the nuclear spin. For the third harmonic of PulsePol, the periodicity is then chosen to be $T = 3\pi/\omega_L$. We adopt this choice here.

Then, by assuming that the transition probabilities $r_\pm \ll 1$ and the time step $\Delta t = T_{\text{tot}} \ll t$ the continuum limit can be taken for our two state model. For nuclear spins with small perpendicular coupling $|A_x| \ll 1/T_{\text{tot}}$ and low

$N_p \leq 4$, these assumptions are valid. The system specific master equations are then

$$\partial_t p_\uparrow(\mathbf{r},t) = u_+(\mathbf{r}) p_\downarrow(\mathbf{r},t) - u_-(\mathbf{r}) p_\uparrow(\mathbf{r},t) + \Gamma p_\downarrow(\mathbf{r},t) - \Gamma p_\uparrow(\mathbf{r},t) \tag{48}$$

$$\partial_t p_\downarrow(\mathbf{r},t) = u_-(\mathbf{r}) p_\uparrow(\mathbf{r},t) - u_+(\mathbf{r}) p_\downarrow(\mathbf{r},t) + \Gamma p_\uparrow(\mathbf{r},t) - \Gamma p_\downarrow(\mathbf{r},t) \tag{49}$$

where $\Gamma = 1/T_1$ is the $T_1$ relaxation rate of the nuclear spin and $u_\pm(\mathbf{r}) = r_\pm/T_{\text{tot}}$. These first order differential equations can be decoupled using the normalisation condition for probability, $p_\uparrow = 1 - p_\downarrow$. Then, the decoupled equation can be re-framed in terms of nuclear spin polarisation using $\mathcal{P} = 1 - 2p_\downarrow$. The differential equation for polarisation accumulation is then

$$\partial_t \mathcal{P} = -(u_+ + u_- + \Gamma)\mathcal{P} + u_+ - u_- \tag{50}$$

where the constant $\Gamma$ has been re-scaled and the dependence on $\mathbf{r}, t$ is implied here. For simplicity, polarisation diffusion due to nuclear spin movement or dipole-dipole coupling has been neglected, where including diffusion introduces terms $-D\nabla^2\mathcal{P}(\mathbf{r},t)$, defining $D$ as the diffusion constant. We find the solution to this differential equation for an initial polarisation of $\mathcal{P}(\mathbf{r},0) = \mathcal{P}_0$ to be

$$\mathcal{P}(\mathbf{r},t) = \mathcal{P}_0 e^{-\alpha(\mathbf{r})t} + \frac{u_+(\mathbf{r}) - u_-(\mathbf{r})}{\alpha(\mathbf{r})}\left(1 - e^{-\alpha(\mathbf{r})t}\right) \tag{51}$$

where $\alpha(\mathbf{r}) = u_+(\mathbf{r}) + u_-(\mathbf{r}) + \Gamma$. As previously stated, the nuclear spin is in a thermal mixture with an initial polarisation $\mathcal{P}_0 = 0$. The asymptotic limit of polarisation for the stationary distribution is then

$$\lim_{t\to\infty} \mathcal{P}(\mathbf{r},t) = \mathcal{P}_\infty(\mathbf{r}) = \frac{r_+(\mathbf{r}) - r_-(\mathbf{r})}{r_+(\mathbf{r}) + r_-(\mathbf{r}) + \Gamma T_{\text{tot}}}. \tag{52}$$

This is similar to that in Eq.(28) with an additional nuclear relaxation term in the denominator.

As with before, we apply the asymptotic polarisation for single nuclear spins in Eq.(52) to $^{13}$C nuclear spins in diamond coupled to a NV center. Although the system and hyperfine couplings are in three dimensions, there is a symmetry of rotations about the $z$-axis by azimuthal angle $\phi$. Therefore, we are free to choose one value of this angle as an example. For simplicity, we choose $\phi = 0$, the $x - z$ plane, such that $\mathbf{r} = X\mathbf{e}_x + Z\mathbf{e}_z$.

For our application, the nuclear spins occupy fixed lattice sites. Hence, the position vector $\mathbf{r}$ is a discrete linear combination of lattice vectors $\{\mathbf{a}_n\}$. The continuum limit can be taken if the distances used satisfy $||\mathbf{r}|| = r \gg a_0$ where $\mathbf{a}_n \cdot \mathbf{a}_m = a_0\delta_{nm}$, the lattice constant. For diamond $a_0 \simeq 3.57$ Å. Moreover, as this is a lattice, the nuclear spins are static and cannot diffuse; however, dipole-dipole mediated spin diffusion is possible, but neglected here. We take the nuclear relaxation time to be $T_1 = 1/\Gamma \simeq 1\,\text{s}$.

Figure 2 shows the asymptotic polarisation of a nuclear spin for both the first order and second order PulsePol Hamiltonian at different orientations to the NV center, which is placed at $\mathbf{r} = (0,0,0)^{\text{T}}$. Due to a larger nuclear detuning, or $A_z$, a nuclear spin in close proximity to the NV center is more likely to be effected by depolarisation, as seen with broader dips of no polarisation and overall lower values. Stark loss of polarisation is seen for spins with $r < 1\,\text{nm}$, however, the model is expected to break in this region as $r \sim a_0$.

In both Fig.2(a) and (b) a nuclear spin with $r > 6\,\text{nm}$ does not appear to polarise. Looking at Eq.(52), the boundary of this transition from a polarising regime to a non-polarising regime may occur when $u_+(\mathbf{r}) + u_-(\mathbf{r}) \simeq \Gamma$. For a distant spin where $\delta \simeq 0$, this is simply when $r_+(\mathbf{r}) \simeq \Gamma T_{\text{tot}}$. Moreover, by assuming that $A_x T_{\text{tot}} \ll 1$ and taking the furthest polarisation distance $\mathbf{r} = r_{\text{max}}(1,0,1)^{\text{T}}/\sqrt{2}$, the polarisation boundary distance from the NV is estimated to be

$$r_{\text{max}} \simeq \sqrt[3]{\frac{3\xi\alpha T_{\text{tot}}}{8}\sqrt{\frac{T_1}{T_{\text{tot}}}}} \tag{53}$$

where $\xi = \hbar\mu_0\gamma_e\gamma_c/4\pi$ and $\alpha = 2(2+\sqrt{2})/3\pi$ for the third harmonic of PulsePol. Setting $T_{\text{tot}} \simeq 60\,\mu\text{s}$, the polarisation boundary is estimated to be $r_{\text{max}} \sim 6\,\text{nm}$, aligning with Fig.2. To estimate the number of nuclear spins polarised in diamond, we assume polarisation of independent nuclear spins and so $N_{\text{pol}} = \int \mathcal{P}_\infty(\mathbf{r})\rho(\mathbf{r})\,d^3\mathbf{r}$ where $\rho(\mathbf{r})$ is the nuclear spin density function. As an upper bound, we further assume that the polarisation boundary is sphere radius $r_{\text{max}}$ and the density is uniform with $\rho = \eta n$ where $n \simeq 1.76 \times 10^{29}$ atoms/$m^3$ is the density of carbon spins in

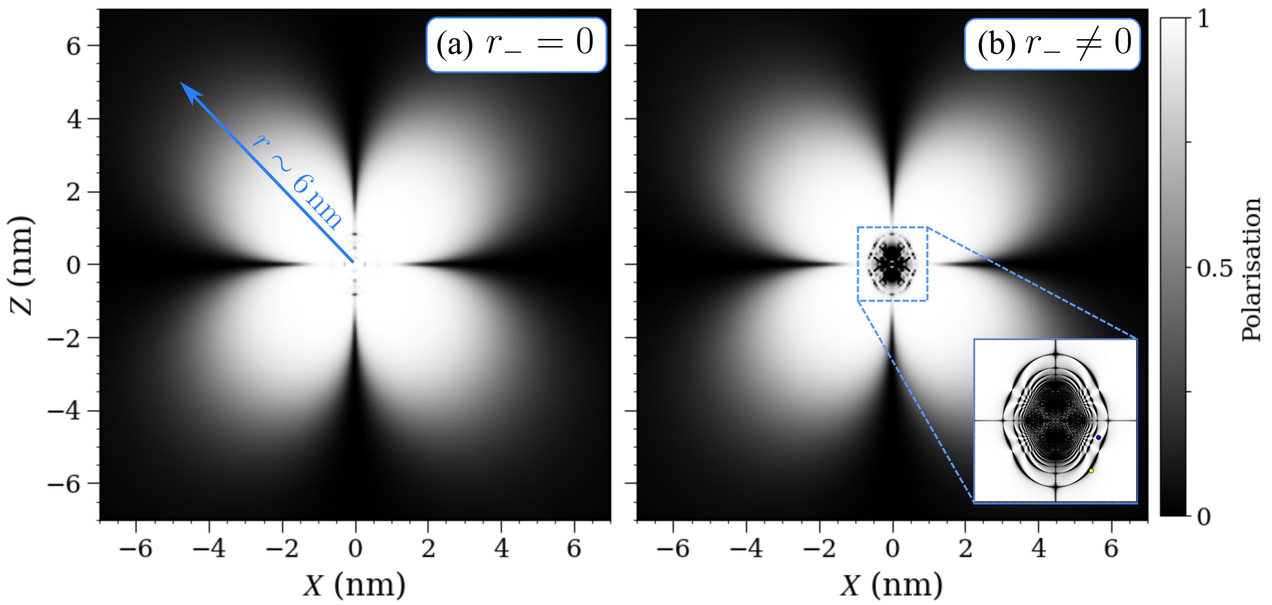


FIG. 2. $^{13}$C asymptotic polarisation via a NV center using PulsePol from Eq.(52) for different orientations $\mathbf{r} = (X, 0, Z)^T$. The periodicity of PulsePol is chosen such that it is resonant with the Larmor precession frequency, or $T = 3\pi/\omega_L$. (a) shows the asymptotic polarisation from Eq.(52) for the first order PulsePol Hamiltonian. As expected, maximal polarisation is met for most orientations where $A_x \neq 0$. However, when the distance from the NV $r > 6\,$nm, no polarisation is seen. (b) now includes the second order terms and de-polarisation $r_-$. The same behaviour is seen at large $r$, but for $r < 2\,$nm, striking regions of no polarisation are seen.

diamond and $\eta \simeq 0.011$ is the natural abundance of $^{13}$C impurities. Then, an upper bound for the number of $^{13}$C spins polarised is

$$N_{\rm pol} < \gamma\alpha T_{\rm tot}\sqrt{\frac{T_1}{T_{\rm tot}}} \sim 2000 \tag{54}$$

where $\gamma = \pi n\eta\xi/2$. Here, $\alpha T_{\rm tot}$ controls the polarisation rate and $\sqrt{T_1/T_{\rm tot}}$ controls the state thermalisation due to relaxation. To increase the number of nuclei polarised, either the relaxation time of the nuclei should be increased, or the polarisation rate; the latter is more readily controlled.


[1] M. H. Abobeih, J. Randall, C. E. Bradley, H. P. Bartling, M. A. Bakker, M. J. Degen, M. Markham, D. J. Twitchen and T. H. Taminiau, *Atomic-scale imaging of a 27-nuclear-spin cluster using a quantum sensor*, Nature, **576**(7787), 411-415 (2019).

[2] G. L. Van de Stolpe, D. P. Kwiatkowski, C. E. Bradley, J. Randall, M. H. Abobeih, S. A. Breitweiser, L. C. Bassett, M. Markham, D. J. Twitchen, and T. H. Taminiau. *Mapping a 50-spin-qubit network through correlated sensing*, Nature Commun. **15**, 1 (2024).

[3] I. Schwartz, J. Scheuer, B. Tratzmiller, S. Muller, Q. Chen, I. Dhand, Z-Y. Wang, C. Muller, B. Naydenov, F. Jelezko, and M. B. Plenio, *Robust optical polarization of nuclear spin baths using Hamiltonian engineering of nitrogen-vacancy center*, Sci. Adv. **4**, eaat8978, (2018).

[4] O.T. Whaites, C.I. Ioannou, B.J. Pingault, G.L. Van De Stolpe, T.H. Taminiau and T.S. Monteiro, *Hyperpolarization of nuclear spins: Polarization blockade*, Phys. Rev. R. **5**(4), p.043291 (2023).
